# Supplementary material for: Few-shot Adaptation of Medical Vision-Language Models
Source: arXiv:2409.03868 source file (2024-09-05)
Supplement: Supplementary file 1 [file 06_Supplementary.tex]

\section{Supplementary Material}

% \paragraph{\textbf{Histology}}Average ACA and std results on 5 tasks for 3 Histology benchmarks.~\ref{table:histo}.

\begin{table*}[ht] 
\footnotesize
\tiny
\centering

\begin{tabular}{l|l|ccccc}
\hline
 Dataset & \textbf{Number of shots ($S$)} & \textbf{1} & \textbf{2} & \textbf{4} & \textbf{8} & \textbf{16}\\
\hline
\hline
\multirow{8}{*}{\textit{NCT-CRC}} & Zero-shot$_\text{ ICML'21}$\cite{radford2021clip} & \multicolumn{5}{c}{60.25}\\
\cline{2-7}
& CoOp$_\text{ IJCV'22}$\cite{Zhou2022coop} & $57.74 \pm10.20$ & $74.58 \pm7.30$ & $83.55 \pm2.94$ & $86.80 \pm0.69$  &  $90.90 \pm1.21$ \\
& CoCoOp$_\text{ CVPR'22}$\cite{zhou2022cocoop} & $62.80 \pm7.12$ & $74.08 \pm4.55$  &  $82.69 \pm2.46$  &  $87.27 \pm0.89$ &  $89.77 \pm1.52$\\
& KgCoOp$_\text{ CVPR'23}$\cite{Yao2023kgcoop} & $68.08 \pm6.65$ & $77.80 \pm3.94$ & $86.22 \pm0.97$ & $86.85 \pm1.62$ & $90.86 \pm0.70$\\
\cline{2-7}
%Tip-Adapter\cite{zhang2022tip} & $60.48\pm0.08$ & $60.56\pm0.16$ & $61.02\pm0.12$ & $61.24\pm0.08$ & $61.59\pm0.10$ \\
%\hline
& CLIP-Adapter$_\text{ IJCV'23}$\cite{Gao2023clipadapter} & $67.52 \pm10.27$ & $77.82 \pm4.05$ & $85.72 \pm2.88$ & $88.43 \pm1.33$ & $89.55 \pm1.53$ \\
& Tip-Adapter-F$_\text{ ECCV'22}$\cite{zhang2022tip} & $75.60 \pm4.06$ & $78.25 \pm2.89$ &  $85.72\pm 0.97$ & $88.73\pm 1.07$  & $91.58\pm 0.99$ \\
%\textcolor{blue}{(-0.48)}
\cline{2-7}
& Linear Probe (LP)$_\text{ ICML'21}$\cite{radford2021clip} & $70.84 \pm 3.39$  &  $79.21 \pm2.40$  &  $85.44 \pm0.98$  &  $89.11 \pm1.06$  & $91.84 \pm0.76$  \\
& \cellcolor{blue!15}{LP+text} & \cellcolor{blue!15}{$\textbf{76.92} \pm 10.08$} &  \cellcolor{blue!15}{$\textbf{82.81} \pm 2.77$} & \cellcolor{blue!15}{$\textbf{87.42} \pm 5.12$} & \cellcolor{blue!15}{$\textbf{90.49} \pm 2.23$} & \cellcolor{blue!15}{$\textbf{91.98} \pm 1.03$}\\
\hline

\multirow{8}{*}{\textit{SICAPv2}} & Zero-shot$_\text{ ICML'21}$\cite{radford2021clip} & \multicolumn{5}{c}{39.05}\\
\cline{2-7}
& CoOp$_\text{ IJCV'22}$\cite{Zhou2022coop} & $32.39 \pm 11.06$ &  $35.88 \pm 12.37$ & $51.09 \pm 7.61$ & $56.40 \pm 9.15$  &  $66.67 \pm 1.75$ \\
& CoCoOp$_\text{ CVPR'23}$\cite{Zhou2022coop} &  $36.07 \pm 9.24$ & $39.94 \pm 7.85$ & $49.20 \pm 4.13$ & $53.25 \pm 3.97$ &  $54.62 \pm 4.63$ \\
& KgCoOp$_\text{ CVPR'23}$\cite{Yao2023kgcoop} & $39.85 \pm 3.22$ & $48.04 \pm 3.48$ & $50.30 \pm 4.89$ & $63.17 \pm 2.28$ & $68.79 \pm 1.34$\\
\cline{2-7}
%Tip-Adapter\cite{zhang2022tip} & $60.48\pm0.08$ & $60.56\pm0.16$ & $61.02\pm0.12$ & $61.24\pm0.08$ & $61.59\pm0.10$ \\
%\hline
& CLIP-Adapter$_\text{ IJCV'23}$\cite{Gao2023clipadapter} & $34.29 \pm 9.44$ & $49.10 \pm 5.04$ & $52.52 \pm 6.31$ & $63.02 \pm 3.56$ & $\textbf{71.78} \pm 0.93$ \\
& Tip-Adapter-F$_\text{ ECCV'22}$\cite{zhang2022tip} & $32.95 \pm 8.94$  & $50.39 \pm 4.14$  & $49.67 \pm 6.67$ & $64.49 \pm 3.94$ & $69.56 \pm 1.45$ \\
%\textcolor{blue}{(-0.48)}
\cline{2-7}
& Linear Probe (LP)$_\text{ ICML'21}$\cite{radford2021clip} & $38.21 \pm 6.26$  &  $\textbf{52.92} \pm2.19$  &  $52.82 \pm5.75$  &  $\textbf{65.25} \pm2.18$  & $69.64 \pm1.82$  \\
& \cellcolor{blue!15}{LP+text} & \cellcolor{blue!15}{$\textbf{40.00} \pm 2.30$} & \cellcolor{blue!15}{$50.27 \pm 4.70$} & \cellcolor{blue!15}{$\textbf{52.99} \pm 3.71$} & \cellcolor{blue!15}{$63.65 \pm 3.26$} & \cellcolor{blue!15}{$70.74 \pm 2.72$}\\
\hline

\multirow{8}{*}{\textit{SkinCancer}} & Zero-shot$_\text{ ICML'21}$\cite{radford2021clip} & \multicolumn{5}{c}{45.69}\\
\cline{2-7}
& CoOp$_\text{ IJCV'22}$\cite{Zhou2022coop} & $48.02 \pm 7.81$ & $53.18 \pm 3.45$ &  $63.49 \pm 3.62$ &  $71.14 \pm 2.72$ &  $75.49 \pm 0.9$ \\
& CoCoOp$_\text{ CVPR'22}$\cite{zhou2022cocoop} & $41.02 \pm6.50$ & $ 53.91 \pm 3.68$ & $64.29 \pm 2.16$ &  $69.61 \pm 3.36$  &  $76.81 \pm 0.57$\\
& KgCoOp$_\text{ CVPR'23}$\cite{Yao2023kgcoop} & $53.95 \pm 7.18$  & $61.48 \pm 2.98$ & $71.58 \pm 2.90$ & $\textbf{78.01} \pm 3.22$ & $80.08 \pm 1.08$ \\
\cline{2-7}
%Tip-Adapter\cite{zhang2022tip} & $60.48\pm0.08$ & $60.56\pm0.16$ & $61.02\pm0.12$ & $61.24\pm0.08$ & $61.59\pm0.10$ \\
%\hline
& CLIP-Adapter$_\text{ IJCV'23}$\cite{Gao2023clipadapter} & $\textbf{55.69} \pm 3.53$ & $60.82 \pm 2.79$ & $69.38 \pm 3.33$ & $76.32 \pm 2.01$ & $80.08 \pm 1.39$ \\
& Tip-Adapter-F$_\text{ ECCV'22}$\cite{zhang2022tip} & $53.35 \pm 2.52$ & $\textbf{61.98} \pm 3.05$ & $\textbf{71.95} \pm 2.92$ & $77.81 \pm 1.54$ & $80.93 \pm 1.72$ \\
%\textcolor{blue}{(-0.48)}
\cline{2-7}
& Linear Probe (LP)$_\text{ ICML'21}$\cite{radford2021clip} & $47.09 \pm 3.82$ & $57.85 \pm 4.57$   & $69.41 \pm 3.81$   &  $75.55 \pm 1.56$  & $79.92 \pm 1.96$  \\
& \cellcolor{blue!15}{LP+text} & \cellcolor{blue!15}{$49.89 \pm 3.24$} & \cellcolor{blue!15}{$60.98 \pm 3.21$} & \cellcolor{blue!15}{$71.26 \pm 2.58$} & \cellcolor{blue!15}{$75.41 \pm 1.48$} & \cellcolor{blue!15}{$\textbf{81.05} \pm 0.89$}\\
\hline

%\multirow{10}{*}{\textit{Camelyon}} & Zero-shot CLIP$_\text{ ICML'21}$\cite{radford2021clip} & \multicolumn{5}{c}{65.19}\\
%\cline{2-7}
%& CoOp$_\text{ IJCV'22}$\cite{Zhou2022coop} & &  &   &  &   \\
%& CoCoOp$_\text{ CVPR'23}$\cite{Yao2023kgcoop} &  &  &  &    &  \\
%& ProGrad$_\text{ ICCV'23}$\cite{Zhu2023prograd} &   &  &  &  & \\
%\cline{2-7}
%Tip-Adapter\cite{zhang2022tip} & $60.48\pm0.08$ & $60.56\pm0.16$ & $61.02\pm0.12$ & $61.24\pm0.08$ & $61.59\pm0.10$ \\
%\hline
%& CLIP-Adapter$_\text{ IJCV'23}$\cite{Gao2023clipadapter} & &  &  &  & \\
%& Tip-Adapter-F$_\text{ ECCV'22}$\cite{zhang2022tip} &  &  &  &  &  \\
%& Tip-Adapter-F*$_\text{ ECCV'22}$\cite{zhang2022tip} &  &  &  &  &  \\
%\textcolor{blue}{(-0.48)}
%\cline{2-7}
%& Linear Probe (LP)$_\text{ ICML'21}$\cite{radford2021clip} &  &    &   &    &   \\
%& \cellcolor{blue!15}{LP+text} & \cellcolor{blue!15}{} & \cellcolor{blue!15}{} & \cellcolor{blue!15}{} & \cellcolor{blue!15}{} & \cellcolor{blue!15}{}\\
%\hline
   
\end{tabular}
    \caption{\textbf{Comparison of state-of-the-art methods}  Average classification accuracy (\%) and standard deviation over 5 tasks for Histology benchmarks. %averaged over the 11 classification benchmarks, 
    Best values are highlighted in bold.} 
    \label{table:histo}
\end{table*}

% \paragraph{\textbf{Ophthalmology}}Average ACA and std results on 5 tasks for 3 Ophthalmology benchmarks.~\ref{table:Ophthalmology}.
\vspace{-1cm}

\begin{table*}[ht] 
\footnotesize
\tiny
\centering

\begin{tabular}{l|l|ccccc}
\hline
 Dataset & \textbf{Number of shots ($S$)} & \textbf{1} & \textbf{2} & \textbf{4} & \textbf{8} & \textbf{16}\\
\hline
\hline
\multirow{10}{*}{\textit{MESSIDOR}} & Zero-shot$_\text{ ICML'21}$\cite{radford2021clip} & \multicolumn{5}{c}{$57.63 \pm 4.84$}\\
\cline{2-7}
& CoOp$_\text{ IJCV'22}$\cite{Zhou2022coop} & $42.11 \pm 11.78$ & $43.67 \pm 5.60$ & $50.60 \pm 11.84$  & $51.36 \pm 4.80$ & $61.35 \pm 2.36$  \\
& CoCoOp$_\text{ CVPR'22}$\cite{chen2023plot} &  $42.57 \pm 15.94$  &  $52.06 \pm 9.82$ & $60.61 \pm 2.60$ & $59.49 \pm 5.35$  & $60.62 \pm 2.55$  \\
& KgCoOp$_\text{ CVPR'23}$\cite{Zhu2023prograd} & $44.25 \pm 10.64$  &  $52.85 \pm 7.75$ & $59.50 \pm 6.76$ & $53.96 \pm 8.12$  & $63.98 \pm 2.38$  \\
\cline{2-7}
%Tip-Adapter\cite{zhang2022tip} & $60.48\pm0.08$ & $60.56\pm0.16$ & $61.02\pm0.12$ & $61.24\pm0.08$ & $61.59\pm0.10$ \\
%\hline
& CLIP-Adapter$_\text{ IJCV'23}$\cite{Gao2023clipadapter}& $59.97 \pm 6.18$ & $62.01 \pm 4.95$ & $61.88 \pm 4.60$ & $\textbf{65.65} \pm 5.01$ & $68.71 \pm 3.47$ \\
& Tip-Adapter-F$_\text{ ECCV'22}$\cite{zhang2022tip} & $\textbf{61.47} \pm 6.10$ & $65.42 \pm 1.87$ & $63.12 \pm 3.70$ & $65.10 \pm 5.87$ & $67.74 \pm 3.62$ \\
%\textcolor{blue}{(-0.48)}
\cline{2-7}
& Linear Probe (LP)$_\text{ ICML'21}$\cite{radford2021clip} & $51.55 \pm 8.73$ & $56.75 \pm 4.35$ & $60.23 \pm 4.42$ & $61.73 \pm 4.78$ & $\textbf{69.42} \pm 3.10$ \\
& \cellcolor{blue!15}{LP+text} & \cellcolor{blue!15}{$58.59 \pm 5.12$} & \cellcolor{blue!15}{$\textbf{62.71} \pm 4.79$} & \cellcolor{blue!15}{$\textbf{63.29} \pm 5.74$} & \cellcolor{blue!15}{$64.72 \pm 3.36$} & \cellcolor{blue!15}{$66.62 \pm 2.74$}\\
\hline

\multirow{10}{*}{\textit{FIVES}} & Zero-shot$_\text{ ICML'21}$\cite{radford2021clip} & \multicolumn{5}{c}{$73.75 \pm 1.42$}\\
\cline{2-7}
& CoOp$_\text{ IJCV'22}$\cite{Zhou2022coop} &$45.00 \pm 9.07$ & $47.50 \pm 7.75$ & $55.50 \pm 7.53$  & $63.63 \pm 4.72$ & $73.50 \pm 1.66$  \\
& CoCoOp$_\text{ CVPR'22}$\cite{chen2023plot} & $42.87 \pm 8.07$  & $59.50 \pm 6.65$  & $70.37 \pm 4.90$  &  $74.00 \pm 3.06$ &  $76.37 \pm 3.59$ \\
& KgCoOp$_\text{CVPR'23}$\cite{Zhu2023prograd} &  $43.63 \pm 11.26$  & $53.25 \pm 13.81$  & $69.75 \pm 6.87$  &  $73.38 \pm 1.09$ &  $78.00 \pm 2.60$ \\
\cline{2-7}
%Tip-Adapter\cite{zhang2022tip} & $60.48\pm0.08$ & $60.56\pm0.16$ & $61.02\pm0.12$ & $61.24\pm0.08$ & $61.59\pm0.10$ \\
%\hline
& CLIP-Adapter$_\text{ IJCV'23}$\cite{Gao2023clipadapter} &  $73.75 \pm 1.72$  & $73.50 \pm 2.55$  & $\textbf{74.75} \pm 3.48$  & $76.00 \pm 2.97$  &  $77.25 \pm 3.07$ \\
& Tip-Adapter-F$_\text{ ECCV'22}$\cite{zhang2022tip} & $72.88 \pm 2.11$  & $73.63 \pm 2.48$  &  $73.87 \pm 1.27$  & $76.50 \pm 2.46$  &  $76.50 \pm 2.36$ \\
%\textcolor{blue}{(-0.48)}
\cline{2-7}
& Linear Probe (LP)$_\text{ ICML'21}$\cite{radford2021clip} & $69.12 \pm 1.09$  &  $\textbf{69.62} \pm 6.78$  &  $74.00 \pm 3.08$ & $\textbf{77.38} \pm 4.22$  & $\textbf{81.75} \pm 2.14$  \\
& \cellcolor{blue!15}{LP+text} & \cellcolor{blue!15}{$\textbf{69.75} \pm5.21$} & \cellcolor{blue!15}{$67.75\pm 6.96$} & \cellcolor{blue!15}{$\textbf{74.38} \pm 2.27$} & \cellcolor{blue!15}{$\textbf{77.25} \pm 2.15$} & \cellcolor{blue!15}{$77.13 \pm2.04$}\\
\hline

\multirow{10}{*}{\textit{ODIR200x3}} & Zero-shot$_\text{ ICML'21}$\cite{radford2021clip} & \multicolumn{5}{c}{$ 65.83 \pm 3.84$}\\
\cline{2-7}
& CoOp$_\text{ IJCV'22}$\cite{Zhou2022coop} & $50.83 \pm 15.16$  &  $59.17 \pm 19.01$ & $69.33 \pm 13.16$  & $71.00 \pm 9.99$  & $82.50 \pm 2.04$  \\
& CoCoOp$_\text{ CVPR'22}$\cite{chen2023plot} &  $58.17 \pm 10.87$  &  $66.00 \pm 7.06$ & $76.50 \pm 8.36$  & $82.33 \pm 4.58$  & $\textbf{88.50} \pm 2.60$  \\
& KgCoOp$_\text{ CVPR'23}$\cite{Zhu2023prograd} & $58.50 \pm 11.13$  &  $74.00 \pm 7.93$ & $80.83 \pm 2.11$  & $81.83 \pm 4.36$  & $84.50 \pm 4.17$  \\
\cline{2-7}
%Tip-Adapter\cite{zhang2022tip} & $60.48\pm0.08$ & $60.56\pm0.16$ & $61.02\pm0.12$ & $61.24\pm0.08$ & $61.59\pm0.10$ \\
%\hline
& CLIP-Adapter$_\text{ IJCV'23}$\cite{Gao2023clipadapter} &  $64.83 \pm 4.55$ &  $68.50 \pm 4.93$  & $74.50 \pm 8.43$  & $81.17 \pm 3.71$ & $87.00 \pm 0.85$\\
& Tip-Adapter-F$_\text{ ECCV'22}$\cite{zhang2022tip} & $66.50 \pm 2.66$  & $75.67 \pm 5.76$  & $79.50 \pm 5.55$ &  $84.66 \pm 3.23$ & $81.67 \pm 3.94$  \\
%\textcolor{blue}{(-0.48)}
\cline{2-7}
& Linear Probe (LP)$_\text{ ICML'21}$\cite{radford2021clip} & $72.50 \pm 3.98$ & $81.16 \pm 4.33$  & $85.17 \pm 5.33$  & $\textbf{86.17} \pm 3.64$ &  $88.33 \pm 1.49$ \\
& \cellcolor{blue!15}{LP+text} & \cellcolor{blue!15}{$\textbf{80.33} \pm 7.93$} & \cellcolor{blue!15}{$\textbf{83.00} \pm 1.45$} & \cellcolor{blue!15}{$\textbf{86.50} \pm 2.32$} & \cellcolor{blue!15}{$85.00 \pm 4.62$} & \cellcolor{blue!15}{$\textbf{88.50} \pm 1.11$}\\
\hline

\end{tabular}
    \caption{ \textbf{Comparison of state-of-the-art methods}  Average classification accuracy (\%) and standard deviation over 5 tasks for Ophthalmology benchmarks. %averaged over the 11 classification benchmarks, 
    Best values are highlighted in bold.}
    \label{table:Ophthalmology}
\end{table*}

% \paragraph{\textbf{Radiology}}Average ACA and std results on 5 tasks for 3 Ophthalmology benchmarks.~\ref{table:radiology}.

\begin{table*}[ht] 
\footnotesize
\tiny
\centering

\begin{tabular}{l|l|ccccc}
\hline
 Dataset & \textbf{Number of shots ($S$)} & \textbf{1} & \textbf{2} & \textbf{4} & \textbf{8} & \textbf{16}\\
\hline
\hline
\multirow{8}{*}{\textit{CHEXPERT-5x200}} & Zero-shot$_\text{ ICML'21}$\cite{radford2021clip} & \multicolumn{5}{c}{56.10}\\
\cline{2-7}
& CoOp$_\text{ IJCV'22}$\cite{Zhou2022coop} & $21.90 \pm 7.52$ & $27.80 \pm 8.91$ & $37.00 \pm 4.14$  & $49.10 \pm 2.60$ &  $52.90 \pm 4.52$ \\
& CoCoOp$_\text{ CVPR'22}$\cite{chen2023plot} & $23.30 \pm9.45$ & $26.60 \pm 5.98$  &  $36.10 \pm 5.48$   &  $38.60 \pm 5.16$ &  $41.80 \pm 3.50$\\
& KgCoOp$_\text{ CVPR'23}$\cite{Yao2023kgcoop} & $28.40 \pm 4.19$ & $36.80 \pm 4.52$ & $39.90 \pm 3.92$ & $47.70 \pm 2.84$   & $51.60 \pm 3.15$ \\
\cline{2-7}
%Tip-Adapter\cite{zhang2022tip} & $60.48\pm0.08$ & $60.56\pm0.16$ & $61.02\pm0.12$ & $61.24\pm0.08$ & $61.59\pm0.10$ \\
%\hline
& CLIP-Adapter$_\text{ IJCV'23}$\cite{Gao2023clipadapter} & $\textbf{56.00} \pm 2.30$ &$\textbf{55.80} \pm 2.11$  & $\textbf{56.10} \pm 2.82$ & $\textbf{57.70} \pm 3.11$ & $\textbf{58.40} \pm 2.13$ \\
& Tip-Adapter-F$_\text{ ECCV'22}$\cite{zhang2022tip} & $54.40 \pm 2.35$ & $54.60 \pm 2.06$ & $55.20 \pm 6.35$ & $54.80 \pm 3.66$ & $57.00 \pm 2.63$ \\
%\textcolor{blue}{(-0.48)}
\cline{2-7}
& Linear Probe (LP)$_\text{ ICML'21}$\cite{radford2021clip} & $32.40 \pm 5.68$ &   $39.70 \pm 5.16$ & $44.60 \pm 4.40$  &  $49.70 \pm 3.33$  &  $51.70 \pm 5.30$ \\
& \cellcolor{blue!15}{LP+text} & \cellcolor{blue!15}{$49.10 \pm 6.37$} & \cellcolor{blue!15}{$54.50 \pm 2.28$} & \cellcolor{blue!15}{$54.70 \pm 2.94$} & \cellcolor{blue!15}{$\textbf{57.70} \pm 3.17$} & \cellcolor{blue!15}{$58.10 \pm 1.73$}\\
\hline

\multirow{8}{*}{\textit{MIMIC-5x200}} & Zero-shot$_\text{ ICML'21}$\cite{radford2021clip} & \multicolumn{5}{c}{51.50}\\
\cline{2-7}
& CoOp$_\text{ IJCV'22}$\cite{Zhou2022coop} & $23.60 \pm 8.01$ &  $28.90 \pm 11.15$ & $42.50 \pm 9.39$  & $50.10 \pm 4.97$ & $55.20 \pm 5.10$  \\
& CoCoOp$_\text{ CVPR'22}$\cite{chen2023plot} & $25.90 \pm 2.56$ & $29.60 \pm 4.92$  &  $36.50 \pm 4.14$  & $33.50 \pm 6.40$  & $38.20 \pm 4.34$  \\
& KgCoOp$_\text{ CVPR'23}$\cite{Yao2023kgcoop} & $28.80 \pm 6.42$ & $34.30 \pm 7.62$ & $45.40 \pm 5.00$ &  $45.80 \pm 7.33$  & $53.50 \pm 5.09$ \\
\cline{2-7}
%Tip-Adapter\cite{zhang2022tip} & $60.48\pm0.08$ & $60.56\pm0.16$ & $61.02\pm0.12$ & $61.24\pm0.08$ & $61.59\pm0.10$ \\
%\hline
& CLIP-Adapter$_\text{ IJCV'23}$\cite{Gao2023clipadapter} & $\textbf{53.10} \pm 3.41$ & $56.00 \pm 4.06$ & $58.10 \pm 4.12$ & $57.50 \pm 2.55$ & $57.60 \pm 2.73$\\
& Tip-Adapter-F$_\text{ ECCV'22}$\cite{zhang2022tip} & $50.70 \pm 4.23$ & $52.80 \pm 1.86$ & $53.40 \pm 2.92$ & $51.20 \pm 3.19$ & $55.30 \pm 3.26$ \\
%\textcolor{blue}{(-0.48)}
\cline{2-7}
& Linear Probe (LP)$_\text{ ICML'21}$\cite{radford2021clip} & $33.60 \pm 5.28$ &  $35.70 \pm 4.57$  &  $42.90 \pm 6.84$ &  $48.40 \pm 3.31$  &  $52.90 \pm 4.73$ \\
& \cellcolor{blue!15}{LP+text} & \cellcolor{blue!15}{$51.10 \pm 5.68$} & \cellcolor{blue!15}{$\textbf{56.20} \pm 6.03$} & \cellcolor{blue!15}{$\textbf{58.60} \pm 4.42$} & \cellcolor{blue!15}{$\textbf{60.20} \pm 3.44$} & \cellcolor{blue!15}{$\textbf{58.20} \pm 3.97$}\\
\hline

\multirow{8}{*}{\textit{RNSA}} & Zero-shot$_\text{ ICML'21}$\cite{radford2021clip} & \multicolumn{5}{c}{73.50}\\
\cline{2-7}
& CoOp$_\text{ IJCV'22}$\cite{Zhou2022coop} & $67.41 \pm 4.34$ & $65.07 \pm 5.80$ & $70.34 \pm 2.88$  & $72.44 \pm 3.97$ &  $\textbf{78.52} \pm 1.27$ \\
& CoCoOp$_\text{ CVPR'22}$\cite{chen2023plot} & $54.36 \pm 5.56$ &  $64.84 \pm 5.93$ &  $68.18 \pm 9.15$  & $75.46 \pm 4.28$  &  $78.20 \pm 2.20$  \\
& KgCoOp$_\text{ CVPR'23}$\cite{Yao2023kgcoop} & $58.52 \pm 10.43$ & $68.99 \pm 8.55$ & $66.42 \pm 7.60$ &  $73.07 \pm 1.72$  & $77.08 \pm 1.03$ \\
\cline{2-7}
%Tip-Adapter\cite{zhang2022tip} & $60.48\pm0.08$ & $60.56\pm0.16$ & $61.02\pm0.12$ & $61.24\pm0.08$ & $61.59\pm0.10$ \\
%\hline
& CLIP-Adapter$_\text{ IJCV'23}$\cite{Gao2023clipadapter} & $74.28 \pm0.92$ & $74.51 \pm0.55$ & $\textbf{75.30} \pm0.93$ & $\textbf{76.98} \pm1.53$ & $76.46 \pm1.88$\\
& Tip-Adapter-F$_\text{ ECCV'22}$\cite{zhang2022tip} & $74.53 \pm0.24$ &  $74.15 \pm0.86$ &  $74.63 \pm2.18$ &  $74.08 \pm2.98$ &  $75.47 \pm0.90$ \\
%\textcolor{blue}{(-0.48)}
\cline{2-7}
& Linear Probe (LP)$_\text{ ICML'21}$\cite{radford2021clip} & $71.95 \pm3.33$ &  $73.48 \pm3.63$  &   $72.34 \pm1.75$ &  $75.80 \pm2.66$  &  $76.91 \pm4.18$ \\
& \cellcolor{blue!15}{LP+text} & \cellcolor{blue!15}{$\textbf{74.96} \pm1.74$} & \cellcolor{blue!15}{$\textbf{75.61} \pm1.32$} & \cellcolor{blue!15}{$75.06 \pm1.52$} & \cellcolor{blue!15}{$76.51 \pm1.21$} & \cellcolor{blue!15}{$76.16 \pm3.47$}\\
\hline

\end{tabular}
    \vspace{0.1cm}
    \caption{. \textbf{Comparison of state-of-the-art methods}  Average classification accuracy (\%) and standard deviation over 5 tasks for Radiology benchmarks. %averaged over the 11 classification benchmarks, 
    Best values are highlighted in bold.}
    \label{table:radiology}
\end{table*}
