# Supplementary material for: Few-shot Adaptation of Medical Vision-Language Models
Source: arXiv:2409.03868 source file (2024-09-05)
Supplement: Supplementary file 2 [file supp_backup.tex]

\begin{table*}[ht]
\vspace{-5mm}
%\scriptsize
\renewcommand{\arraystretch}{1.2}
\centering
\caption{\textbf{Comparison of state-of-the-art methods.} Average ACA (\%) on 3 benchmarks for each modality Best values are highlighted in bold.} \label{table:avg-main}
\resizebox{1\textwidth}{!}{
\begin{tabular}{clcccccc}
\hline
& \textbf{Number of shots ($S$)} & \textbf{1} & \textbf{2} & \textbf{4} & \textbf{8} & \textbf{16}\\
\hline
\hline
\parbox[t]{2mm}{\multirow{10}{*}{\rotatebox[origin=c]{90}{Histology}}} &Zero-shot $_\text{ ICML'21}$\cite{radford2021clip} & \multicolumn{5}{c}{48.33}\\
\hline
& \textit{Prompt-Learning}& & & & & &\\
%\hdashline
& CoOp$_\text{ IJCV'22}$\cite{Zhou2022coop} & $46.05 \pm 9.79$ & $54.55 \pm 8.53$  &  $66.04 \pm 5.15$  & $71.45 \pm 5.53$  &  $77.69 \pm 1.32$ \\
& CoCoOp$_\text{ CVPR'22}$\cite{chen2023plot} & $46.63 \pm 7.71$ &  $55.98 \pm 5.65$ &  $65.39 \pm 3.04$  & $70.04 \pm 3.05$  & $73.73 \pm 2.83$  \\
& KgCoOp$_\text{ CVPR'23}$\cite{Yao2023kgcoop} & $53.96 \pm 5.95$ & $62.44 \pm 3.49$ & $69.37 \pm 3.33$ &$76.01 \pm 2.46$ & $79.91 \pm 1.07$ \\
\cline{2-7}
& \textit{CLIP-based Adapters} & & & & & \\
%\hdashline
%Tip-Adapter\cite{zhang2022tip} & $60.48\pm0.08$ & $60.56\pm0.16$ & $61.02\pm0.12$ & $61.24\pm0.08$ & $61.59\pm0.10$ \\
%\hline
& CLIP-Adapter$_\text{ IJCV'23}$\cite{Gao2023clipadapter} & $52.50 \pm 8.31 $ & $62.58 \pm 4.07$ & $69.21 \pm 4.44$ & $75.92 \pm 2.48$ & $ 80.47 \pm 1.31$ \\
& Tip-Adapter-F$_\text{ ECCV'22}$\cite{zhang2022tip} & $53.97 \pm6.11$ & $63.54 \pm3.41$ & $69.11 \pm4.24$  & $\textbf{77.01}\pm 2.52$  & $80.69\pm 1.42$ \\
%\textcolor{blue}{(-0.48)}
\cline{2-7}
& Linear Probe (LP)$_\text{ ICML'21}$\cite{radford2021clip} & $52.05 \pm 4.66$  &  $63.33 \pm 3.24$  &  $69.22 \pm4.02$  &  $76.64 \pm1.66$  & $80.47\pm 1.61$  \\
& \cellcolor{blue!15}{LP+text} & \cellcolor{blue!15}{$\textbf{55.60} \pm 6.26$} & \cellcolor{blue!15}{$\textbf{64.69} \pm 3.65$} & \cellcolor{blue!15}{$\textbf{70.56} \pm 3.94$} & \cellcolor{blue!15}{$76.52 \pm 2.44$} & \cellcolor{blue!15}{$\textbf{81.26} \pm 1.76$}\\
\hline
\hline
%%%%%%%%%%%%%%%%%%%%%%%%%%%%%%%%%%%%%%%%%%%%%%%%%%%5
\parbox[t]{2mm}{\multirow{10}{*}{\rotatebox[origin=c]{90}{Ophthalmology}}} & Zero-shot $_\text{ ICML'21}$\cite{radford2021clip} & \multicolumn{5}{c}{65.74}\\
\hline
& \textit{Prompt-Learning}& & & & & &\\
%\hdashline{2-6}
& CoOp$_\text{ IJCV'22}$\cite{Zhou2022coop} & $45.98 \pm 12.26$ & $50.11 \pm 12.29$  &  $58.48 \pm 11.12$  & $62.00 \pm 6.96$  &  $72.45 \pm 2.04$ \\
& CoCoOp$_\text{ CVPR'22}$\cite{chen2023plot} & $47.87 \pm 12.07$ &  $59.19 \pm 7.97$ &  $69.16 \pm 5.79$  &  $71.94 \pm 4.43$ & $77.16 \pm 3.01$  \\
& KgCoOp$_\text{ CVPR'23}$\cite{Yao2023kgcoop} & $46.23 \pm 10.26$ & $55.03 \pm 8.01$ & $62.98 \pm 4.49$ &$64.31 \pm 4.92$ & $71.67 \pm 4.98$ \\
\cline{2-7}
&\textit{CLIP-based Adapters} & & & & & \\
%\hdashline
%Tip-Adapter\cite{zhang2022tip} & $60.48\pm0.08$ & $60.56\pm0.16$ & $61.02\pm0.12$ & $61.24\pm0.08$ & $61.59\pm0.10$ \\
%\hline
&CLIP-Adapter$_\text{ IJCV'23}$\cite{Gao2023clipadapter} & $66.18 \pm 4.54 $ & $68.00 \pm 4.29$ & $70.38 \pm 5.90$ & $74.27 \pm 3.99$ & $ 77.65 \pm 2.72$ \\
& Tip-Adapter-F$_\text{ ECCV'22}$\cite{zhang2022tip} & $66.95 \pm4.03$ & $\textbf{71.57} \pm3.78$ & $72.16 \pm3.92$  & $75.42\pm 4.12$  & $75.30\pm 3.38$ \\
%\textcolor{blue}{(-0.48)}
\cline{2-7}
& Linear Probe (LP)$_\text{ ICML'21}$\cite{radford2021clip} & $64.39 \pm 5.57$  &  $69.18 \pm 5.28$  &  $73.13 \pm4.38$  &  $75.09 \pm4.24$  & $\textbf{79.83}\pm 2.34$  \\
& \cellcolor{blue!15}{LP+text} & \cellcolor{blue!15}{$\textbf{69.56} \pm 6.22$} & \cellcolor{blue!15}{$71.15 \pm 4.95$} & \cellcolor{blue!15}{$\textbf{74.72} \pm 3.80$} & \cellcolor{blue!15}{$\textbf{75.66} \pm 3.42$} & \cellcolor{blue!15}{$77.42 \pm 2.07$}\\
\hline
\hline
%%%%%%%%%%%%%%%%%%%%%%%%%%%%%%%%%%%%%%%%%%%%%%%%%%%%%%%%%%%%%%%%%%%%%%%%%%%%%
\parbox[t]{2mm}{\multirow{10}{*}{\rotatebox[origin=c]{90}{Radiology}}} &Zero-shot $_\text{ ICML'21}$\cite{radford2021clip} & \multicolumn{5}{c}{60.37}\\
\hline
& \textit{Prompt-Learning}& & & & & &\\
%\hdashline
& CoOp$_\text{ IJCV'22}$\cite{Zhou2022coop} & $37.64 \pm 6.82$ & $40.82 \pm 6.76$  &  $49.95 \pm 6.15$  & $57.21 \pm 3.97$  &  $62.21 \pm 4.00$ \\
& CoCoOp$_\text{ CVPR'22}$\cite{chen2023plot} & $34.52 \pm 6.50$ &  $40.35 \pm 5.63$ &  $46.93 \pm 6.60$  &  $49.19 \pm 4.55$ & $52.73 \pm 3.46$  \\
& KgCoOp$_\text{ CVPR'23}$\cite{Yao2023kgcoop} & $38.57 \pm 7.47$ & $46.70 \pm 7.11$ & $50.57 \pm 5.72$ &$55.39 \pm 3.47$ & $60.73 \pm 3.51$ \\
\cline{2-7}
& \textit{CLIP-based Adapters} & & & & & \\
%\hdashline
%Tip-Adapter\cite{zhang2022tip} & $60.48\pm0.08$ & $60.56\pm0.16$ & $61.02\pm0.12$ & $61.24\pm0.08$ & $61.59\pm0.10$ \\
%\hline
& CLIP-Adapter$_\text{ IJCV'23}$\cite{Gao2023clipadapter} & $\textbf{61.13} \pm 2.43 $ & $\textbf{62.10} \pm 2.66$ & $\textbf{63.17} \pm 2.93$ & $64.06 \pm 2.48$ & $ \textbf{64.15} \pm 2.27$ \\
& Tip-Adapter-F$_\text{ ECCV'22}$\cite{zhang2022tip} & $59.88 \pm2.80$ & $60.52 \pm1.68$ & $62.64 \pm4.55$  & $60.03\pm 3.29$  & $62.59\pm 2.47$ \\
%\textcolor{blue}{(-0.48)}
\cline{2-7}
& Linear Probe (LP)$_\text{ ICML'21}$\cite{radford2021clip} & $45.98 \pm 4.87$  &  $49.63 \pm 4.50$  &  $53.28 \pm4.80$  &  $57.97 \pm3.12$  & $60.50\pm 4.76$  \\
& \cellcolor{blue!15}{LP+text} & \cellcolor{blue!15}{$58.39 \pm 5.03$} & \cellcolor{blue!15}{$\textbf{62.10} \pm 3.80$} & \cellcolor{blue!15}{$62.79 \pm 3.19$} & \cellcolor{blue!15}{$\textbf{64.80} \pm 2.79$} & \cellcolor{blue!15}{$\textbf{64.15} \pm 3.20$}\\
\hline
%%%%%%%%%%%%%%%%%%%%%%%%%%%%%%%%%%%%%%%%%%%%%%%%%%%
%%%%%%%%%%%%%%%%%%%%%%%%%%%%%%%%%%%%%%%%%%%%%%%%%%%%%%5

\end{tabular}
 }
\end{table*}
